# Supplementary material for: Parallel Multi Channel Convolution using General Matrix Multiplication
Source: arXiv:1704.04428 source file (2017-07-03)
Supplement: Supplementary file 1 [file appendix.tex]

\begin{appendices}

\section{Dedicated Figures Page}
\label{sec:appendix}

%\begin{figure*}[!ht]
%\centering
%\subfloat[Execution times for all the methods running the convolutional layers of VGG-16 on Ivy Bridge. \textbf{Lower is better}.]{
%\includegraphics[width=.85\linewidth]{results/vgg-16-graphs-x86_64/cyc}
%\label{fig:cyc-vgg-16-ivy}
%}\qquad
%\subfloat[Execution times for all the methods running the convolutional layers of VGG-16 on Tesla K40-GPU. \textbf{Lower is better}.]{
%\includegraphics[width=.85\linewidth]{results/vgg-16-graphs-k40c/cyc}
%\label{fig:cyc-vgg-16-k40gpu}
%}
%
%\caption{Summary of performance of our proposed methods on selected \gls{mcmk} operations from \gls{vgg} on the architectures from Table~\ref{tab:expr-platforms}. Performance is measured
%as the mean execution time over 25 runs of each benchmark. The names used for kernels are those from the Netscope \gls{cnn} Analyzer~\cite{netscope}.}
%\label{fig:cyc-vgg}
%\end{figure*}

\begin{figure*}[!ht]
	\centering
	\resizebox{\linewidth}{!}{
		\subfloat[test1]{
			\includegraphics{results/vgg-16-graphs-x86_64/cyc}
			\label{fig:cyc-vgg-16-ivy}
		}
		\subfloat[test2]{
			\includegraphics{results/googlenet-graphs-x86_64/cyc}
			\label{fig:cyc-vgg-16-ivy}
		}
		\subfloat[test3]{
			\includegraphics{results/alexnet-graphs-x86_64/cyc}
			\label{fig:cyc-vgg-16-ivy}
		}
	}

	\caption{TEST1234}
	\label{fig:cyc-vgg}
\end{figure*}

\begin{figure*}[!ht]
\centering
\subfloat[Execution times for all the methods running the convolutional layers of \gls{alexnet} on Ivy Bridge. \textbf{Lower is better}.]{
\includegraphics[width=0.32\linewidth]{results/alexnet-graphs-x86_64/cyc}
\label{fig:cyc-alex-ivy}
}~
\subfloat[Execution times for all the methods running the convolutional layers of \gls{alexnet} on Tegra TX1-GPU. \textbf{Lower is better}.]{
\includegraphics[width=0.32\linewidth]{results/alexnet-graphs-tx1/cyc}
\label{fig:cyc-alex-tx1gpu}
}~
\subfloat[Execution times for all the methods running the convolutional layers of \gls{alexnet} on Tesla K40-GPU. \textbf{Lower is better}.]{
\includegraphics[width=0.32\linewidth]{results/alexnet-graphs-k40c/cyc}
\label{fig:cyc-alex-k40gpu}
}

\caption{Summary of performance of our proposed methods on selected \gls{mcmk} operations from \gls{alexnet} on the architectures from Table~\ref{tab:expr-platforms}. Performance is measured
as the mean execution time over 25 runs of each benchmark. The names used for kernels are those from the Netscope \gls{cnn} Analyzer~\cite{netscope}.}
\label{fig:cyc-alexnet}
\end{figure*}

%\begin{figure*}[h]
%	\centering
%	\includegraphics[width=.85\linewidth]{results/vgg-16-graphs-tx1/cyc}
%	\caption{Execution times for all the methods running the convolutional layers of VGG-16 on Tegra TX1-GPU}
%	\label{fig:cyc-vgg-16-tx1gpu}
%\end{figure*}

\begin{figure*}[!ht]
\centering
\subfloat[Execution times for all the methods running the convolutional layers of \gls{googlenet} on Ivy Bridge. \textbf{Lower is better}.]{
\includegraphics[width=.85\linewidth]{results/googlenet-graphs-x86_64/cyc}
\label{fig:cyc-googlenet-ivy}
}\qquad
\subfloat[Execution times for all the methods running the convolutional layers of \gls{googlenet} on Tegra TX1-GPU. \textbf{Lower is better}.]{
\includegraphics[width=.85\linewidth]{results/googlenet-graphs-tx1/cyc}
\label{fig:cyc-googlenet-tx1gpu}
}\qquad
\subfloat[Execution times for all the methods running the convolutional layers of \gls{googlenet} on Tesla K40-GPU. \textbf{Lower is better}.]{
\includegraphics[width=.85\linewidth]{results/googlenet-graphs-k40c/cyc}
\label{fig:cyc-googlenet-k40gpu}
}

\caption{Summary of performance of our proposed methods on selected \gls{mcmk} operations from \gls{googlenet} on the architectures from Table~\ref{tab:expr-platforms}. Performance is measured
as the mean execution time over 25 runs of each benchmark. The names used for kernels are those from the Netscope \gls{cnn} Analyzer~\cite{netscope}.}
\label{fig:cyc-googlenet}
\end{figure*}

\end{appendices}
